# Supplementary material for: MACI: Multi-Agent Collaborative Intelligence for Adaptive Reasoning and Temporal Planning
Source: arXiv:2501.16689 source file (2025-01-29)
Supplement: Supplementary file 1 [file AppendixACO.tex]

\subsubsection{ACO-Optimized $\mathbf{W^*}$ Workflow TSP}

\subsection*{3.2.1. Workflow Components}

\paragraph{Nodes ($N$)}
\begin{itemize}[leftmargin=1.2em, topsep=-.15em, parsep=-.15em]
    \item $n_{\text{init}}$: Initializes pheromone trails and heuristic visibility.
    \item $n_{\text{optimize}}$: Constructs tours via ant agents and updates pheromones.
    \item $n_{\text{valid}}$: Validates tour feasibility (starts/ends at A, no repeats).
\end{itemize}

\paragraph{Edges ($E$)}
\begin{itemize}[leftmargin=1.2em, topsep=-.15em, parsep=-.15em]
    \item $e_{\text{pheromone}}$: Pheromone intensity between locations.
    \item $e_{\text{heuristic}}$: Visibility $\eta_{ij} = 1/D_{ij}$ (inverse of distance).
    \item $e_{\text{converge}}$: Monitors solution stability for termination.
\end{itemize}

\paragraph{Agents}
\begin{itemize}[leftmargin=1.2em, topsep=-.15em, parsep=-.15em]
    \item \textbf{Node Agents}:
        \begin{itemize}[leftmargin=1.2em, topsep=-.15em, parsep=-.15em]
            \item $\alpha_{\text{init}}$: Sets initial pheromones $\tau_{ij}(0) = 0.1$.
            \item $\alpha_{\text{ant}}$: 50 ants building tours probabilistically.
            \item $\alpha_{\text{valid}}$: Rejects invalid tours (e.g., missing nodes).
        \end{itemize}
    \item \textbf{Edge Agents}:
        \begin{itemize}[leftmargin=1.2em, topsep=-.15em, parsep=-.15em]
            \item $\alpha_{\text{evap}}$: Evaporates pheromones ($\tau_{ij} \leftarrow 0.9\tau_{ij}$).
            \item $\alpha_{\text{update}}$: Deposits pheromones on best tours.
        \end{itemize}
\end{itemize}

\subsection*{3.2.2. Solution Steps}

\paragraph{Step 1: Initialization ($n_{\text{init}}$)}
\begin{itemize}[leftmargin=1.2em, topsep=-.15em, parsep=-.15em]
    \item Set initial pheromones: $\tau_{ij}(0) = 0.1$ for all edges.
    \item Compute heuristic visibility: $\eta_{ij} = \frac{1}{D_{ij}}$ (e.g., $\eta_{AD} = 1/4 = 0.25$).
\end{itemize}

\paragraph{Step 2: Tour Construction ($n_{\text{optimize}}$)}
\begin{itemize}[leftmargin=1.2em, topsep=-.15em, parsep=-.15em]
    \item Each ant builds a tour incrementally:
        \[
        P_{ij} = \frac{[\tau_{ij}]^1 [\eta_{ij}]^2}{\sum_{l} [\tau_{il}]^1 [\eta_{il}]^2}
        \]
    \item Example ant paths (no full enumeration):
        \begin{itemize}[leftmargin=1.2em, topsep=-.15em, parsep=-.15em]
            \item Ant 1: $A \xrightarrow{55\%} D \xrightarrow{70\%} B \xrightarrow{60\%} C \xrightarrow{80\%} E \to A$ (24 mins)
            \item Ant 2: $A \xrightarrow{45\%} B \xrightarrow{65\%} D \xrightarrow{50\%} C \xrightarrow{75\%} E \to A$ (24 mins)
        \end{itemize}
\end{itemize}

\paragraph{Step 3: Pheromone Update ($e_{\text{pheromone}}$)}
\begin{itemize}[leftmargin=1.2em, topsep=-.15em, parsep=-.15em]
    \item Evaporate pheromones: $\tau_{ij} \leftarrow 0.9 \cdot \tau_{ij}$.
    \item Deposit pheromones on edges of the best tour:
        \[
        \tau_{ij} \leftarrow \tau_{ij} + \frac{10}{24} \quad \text{(e.g., for 24-minute tour)}
        \]
\end{itemize}

\paragraph{Step 4: Validation ($n_{\text{valid}}$)}
\begin{itemize}[leftmargin=1.2em, topsep=-.15em, parsep=-.15em]
    \item Check ant-generated tours for:
        \begin{itemize}[leftmargin=1.2em, topsep=-.15em, parsep=-.15em]
            \item Start/end at A.
            \item All 5 locations visited.
        \end{itemize}
    \item Discard invalid tours (e.g., $A \to B \to C \to D \to A$ misses E).
\end{itemize}

\paragraph{Step 5: Convergence Check ($e_{\text{converge}}$)}
\begin{itemize}[leftmargin=1.2em, topsep=-.15em, parsep=-.15em]
    \item Terminate after 20 iterations or if best tour doesn’t improve for 5 steps.
\end{itemize}

\subsection*{3.2.3. Performance Analysis}

\begin{tabular}{lll}
\toprule
\textbf{Metric} & \textbf{Brute Force} & \textbf{ACO} \\
\midrule
Routes Eval. & 12 (all permutations) & 50 ants $\times$ 20 iterations = 1,000 \\
Operations & 60 edge checks & 1,000 $\times$ 5 edges = 5,000 \\
Complexity & $\mathcal{O}(n!)$ & $\mathcal{O}(Kn^2)$ \\
Result & Guaranteed optimal & Approximate (optimal in this case) \\
\bottomrule
\end{tabular}

\subsection*{3.2.4. Optimal Solution}
Three shortest paths (24 mins) emerge from pheromone reinforcement:  
\begin{itemize}[leftmargin=1.2em, topsep=-.15em, parsep=-.15em]
    \item $A \rightarrow D \rightarrow B \rightarrow C \rightarrow E \rightarrow A$  
    \item $A \rightarrow B \rightarrow D \rightarrow C \rightarrow E \rightarrow A$  
    \item $A \rightarrow E \rightarrow C \rightarrow B \rightarrow D \rightarrow A$  
\end{itemize}

\boxed{24 \text{ minutes (e.g., } A \rightarrow D \rightarrow B \rightarrow C \rightarrow E \rightarrow A)}
