# Supplementary material for: MACI: Multi-Agent Collaborative Intelligence for Adaptive Reasoning and Temporal Planning
Source: arXiv:2501.16689 source file (2025-01-29)
Supplement: Supplementary file 2 [file AppendixAMetaPlanning.tex]

\section{MACI Agent Architecture with Temporal Planning Tools Integration}
\label{app:MACIAgent4Temporal}

\subsection{Overview}
We propose integrating established temporal planning tools into MACI through specialized agents, each leveraging proven algorithms while adding LLM-based reasoning capabilities.

\begin{verbatim}
MACI
+-- Planning Agents
|   +--- Constraint Identification Agent
|   +--- Resource Analysis Agent
|   +--- Validation Agent
+-- Scheduling Engine (STN/DTN)
+-- Execution Monitoring    
\end{verbatim}

\subsection{Core Planning Agents}

\subsubsection{Constraint Management Agent}
Built on Simple Temporal Networks (STN):
\begin{itemize}
   \item \textbf{Base Capability}: STN for basic temporal constraint representation
   \item \textbf{Enhanced Features}:
       \begin{itemize}
           \item LLM-powered implicit constraint identification
           \item Common sense validation of constraints
           \item Dynamic constraint updating based on context
       \end{itemize}
   \item \textbf{Implementation}: Extend NetworkX or specialized STN libraries
\end{itemize}

\subsubsection{Advanced Scheduling Agent}
Built on Disjunctive Temporal Networks (DTN):
\begin{itemize}
   \item \textbf{Base Capability}: DTN for handling alternative scheduling paths
   \item \textbf{Enhanced Features}:
       \begin{itemize}
           \item Alternative path reasoning
           \item Schedule optimization with context awareness
           \item Risk assessment of different scheduling options
       \end{itemize}
   \item \textbf{Implementation}: Custom DTN implementation with LLM integration
\end{itemize}

\subsubsection{Resource Management Agent}
Built on Resource-Constrained Project Scheduling (RCPS):
\begin{itemize}
   \item \textbf{Base Capability}: RCPS algorithms for resource allocation
   \item \textbf{Enhanced Features}:
       \begin{itemize}
           \item Intelligent resource conflict resolution
           \item Priority-based allocation strategies
           \item Dynamic resource reallocation
       \end{itemize}
   \item \textbf{Implementation}: Extend OR-Tools with custom constraints
\end{itemize}

\subsection{Supporting Agents}

\subsubsection{Validation Agent}
\begin{itemize}
   \item Cross-check constraints across different temporal networks
   \item Verify resource allocation feasibility
   \item Monitor for constraint violations
   \item Generate explanation of validation results
\end{itemize}

\subsubsection{Risk Assessment Agent}
Built on Probabilistic Temporal Networks:
\begin{itemize}
   \item Analyze schedule uncertainties
   \item Generate risk mitigation strategies
   \item Provide confidence metrics for plans
\end{itemize}

\subsection{Integration Architecture}

\subsubsection{Communication Protocol}
\begin{itemize}
   \item Standardized constraint representation
   \item Event-driven updates
   \item Priority-based message handling
\end{itemize}

\subsubsection{Data Flow}
\begin{verbatim}
Input Request -> Constraint Agent -> Scheduling Agent
                    ^                    ^
                    |                    |
                    v                    v
             Resource Agent  <->  Validation Agent
                    ^                    ^
                    |                    |
                    v                    v
             Risk Assessment  ->   Final Plan

\end{verbatim}

\subsection{Development Phases}

\subsubsection{Phase 1: Core Implementation}
\begin{itemize}
   \item Implement base temporal network integrations
   \item Develop basic agent communication
   \item Create simple validation mechanisms
\end{itemize}

\subsubsection{Phase 2: Enhanced Features}
\begin{itemize}
   \item Add LLM reasoning capabilities
   \item Implement advanced validation
   \item Develop risk assessment
\end{itemize}

\subsubsection{Phase 3: Application Integration}
\begin{itemize}
   \item Financial planning specific features
   \item Project planning adaptations
   \item Domain-specific optimizations
\end{itemize}

\subsection{Evaluation Metrics}
\begin{itemize}
   \item Constraint satisfaction accuracy
   \item Plan feasibility rate
   \item Resource utilization efficiency
   \item Risk prediction accuracy
\end{itemize}

\subsection{Expected Advantages}
\begin{itemize}
   \item Combines proven scheduling algorithms with LLM reasoning
   \item Maintains mathematical rigor while adding flexibility
   \item Enables explanation and justification of plans
   \item Provides multiple validation layers
\end{itemize}
