# Supplementary material for: MACI: Multi-Agent Collaborative Intelligence for Adaptive Reasoning and Temporal Planning
Source: arXiv:2501.16689 source file (2025-01-29)
Supplement: Supplementary file 3 [file AppendixBCodingGuide.tex]

\section{$\MACI$ Implementation Guide}
\label{app:MACIGuide}

\subsection{Initial Setup}
First, create repository and basic structure:

\begin{verbatim}
# Create repository
git init maci-framework
cd maci-framework

# Create directory structure
mkdir -p src/core src/agents src/api tests
touch src/__init__.py
touch src/core/{__init__.py,auth.py,config.py,message.py}
touch src/agents/{__init__.py,base.py,registry.py}
touch src/api/{__init__.py,endpoints.py}

# Create setup.py for package management
touch setup.py
\end{verbatim}

\subsection{Core Components}

\subsubsection{Message Protocol}
The message protocol defines communication between agents:
\begin{verbatim}
# src/core/message.py
from pydantic import BaseModel
from typing import Any, Optional
from enum import Enum

class MessageType(Enum):
   HELLO = "hello"
   TASK = "task"
   RESPONSE = "response"
   ERROR = "error"

class Message(BaseModel):
   source_id: str
   target_id: str
   message_type: MessageType
   content: Any
   priority: Optional[int] = 1
\end{verbatim}

\subsubsection{LLM Interface}
Abstract interface for LLM integration:
\begin{verbatim}
# src/core/llm.py
from abc import ABC, abstractmethod
from typing import Any

class LLMInterface(ABC):
   """Abstract interface for LLM integration"""
   @abstractmethod 
   async def generate(self, prompt: str) -> str:
       pass

class MockLLM(LLMInterface):
   """Mock LLM for testing"""
   async def generate(self, prompt: str) -> str:
       return "mock response"
\end{verbatim}

\subsubsection{Base Agent}
Template for all MACI agents:
\begin{verbatim}
# src/agents/base.py
from abc import ABC, abstractmethod
from ..core.message import Message, MessageType
from ..core.llm import LLMInterface

class BaseAgent(ABC):
   """Base class for all MACI agents"""
   def __init__(self, agent_id: str,
       capabilities: list[str], llm:LLMInterface):
       self.agent_id = agent_id
       self.capabilities = capabilities
       self.llm = llm

   @abstractmethod
   async def process_message(self, message: Message) -> Message:
       pass

   async def hello(self) -> Message:
       return Message(
           source_id=self.agent_id,
           target_id="*",
           message_type=MessageType.HELLO,
           content=f"Agent {self.agent_id} 
              ready with capabilities: {self.capabilities}"
       )
\end{verbatim}

\subsubsection{Example Agent}
Implementation of a simple agent:
\begin{verbatim}
# src/agents/example.py
from .base import BaseAgent
from ..core.message import Message, MessageType

class HelloAgent(BaseAgent):
   """Simple agent that responds to hello messages"""
   async def process_message(self, message: Message) -> Message:
       if message.message_type == MessageType.HELLO:
           return Message(
               source_id=self.agent_id,
               target_id=message.source_id,
               message_type=MessageType.RESPONSE,
               content=f"Hello {message.source_id}, 
                  I am {self.agent_id}"
           )
       return Message(
           source_id=self.agent_id,
           target_id=message.source_id,
           message_type=MessageType.ERROR,
           content="Unsupported message type"
       )
\end{verbatim}

\subsubsection{Agent Registry}
Central registry for managing agents:
\begin{verbatim}
# src/core/registry.py
from typing import Dict
from ..agents.base import BaseAgent
from ..core.message import Message

class AgentRegistry:
   """Central registry for MACI agents"""
   def __init__(self):
       self._agents: Dict[str, BaseAgent] = {}

   async def register(self, agent: BaseAgent) -> None:
       if agent.agent_id in self._agents:
           raise ValueError(f"Agent {agent.agent_id} already registered")
       self._agents[agent.agent_id] = agent
       
   async def get_agent(self, agent_id: str) -> BaseAgent:
       if agent_id not in self._agents:
           raise ValueError(f"Agent {agent_id} not found")
       return self._agents[agent_id]
\end{verbatim}

\subsubsection*{B.2.6 API Endpoints}
FastAPI endpoints for agent interaction:
\begin{verbatim}
# src/api/endpoints.py
from fastapi import FastAPI, HTTPException
from pydantic import BaseModel
from ..core.registry import AgentRegistry
from ..core.message import Message, MessageType
from ..agents.example import HelloAgent
from ..core.llm import MockLLM

class AgentRegistration(BaseModel):
   agent_id: str
   capabilities: list[str]

class MessageRequest(BaseModel):
   source_id: str
   target_id: str
   message_type: str
   content: str
   priority: int = 1

app = FastAPI()
registry = AgentRegistry()

@app.post("/agent/register")
async def register_agent(registration: AgentRegistration):
   try:
       agent = HelloAgent(
           agent_id=registration.agent_id,
           capabilities=registration.capabilities,
           llm=MockLLM()
       )
       await registry.register(agent)
       return {"status": "success", "message": 
          f"Agent {registration.agent_id} registered"}
   except ValueError as e:
       raise HTTPException(status_code=400, detail=str(e))

@app.post("/agent/message")
async def send_message(msg: MessageRequest):
   try:
       message = Message(
           source_id=msg.source_id,
           target_id=msg.target_id,
           message_type=MessageType(msg.message_type),
           content=msg.content,
           priority=msg.priority
       )
       target_agent = await registry.get_agent(message.target_id)
       response = await target_agent.process_message(message)
       return response
   except ValueError as e:
       raise HTTPException(status_code=404, detail=str(e))
\end{verbatim}

\subsection{Running the System}
Start the server:
\begin{verbatim}
uvicorn src.api.endpoints:app --reload
\end{verbatim}

Test with curl commands:
\begin{verbatim}
# Register agent
curl -X POST "http://localhost:8000/agent/register" \
    -H "Content-Type: application/json" \
    -d '{"agent_id": "agent1", "capabilities": ["hello"]}'

# Send message
curl -X POST "http://localhost:8000/agent/message" \
    -H "Content-Type: application/json" \
    -d '{"source_id": "test", "target_id": "agent1", \
        "message_type": "hello", "content": 
        "Hello!", "priority": 1}'
\end{verbatim}

\subsection{Key Design Decisions}
\begin{itemize}
\item Asynchronous communication using FastAPI
\item Modular agent architecture with dependency injection
\item Type safety using Pydantic models
\item Centralized registry for agent management
\item Clear separation of concerns between components
\end{itemize}

\subsection{Project Structure}

The complete project structure:
\begin{verbatim}
maci-framework/
+ src/
|   + core/
|   |   + __init__.py
|   |   + auth.py        # Authentication (future)
|   |   + config.py      # Configuration
|   |   + llm.py         # LLM interface
|   |   + message.py     # Message protocols
|   |   + registry.py    # Agent registry
|   | agents/
|   |   + __init__.py
|   |   + base.py        # Base agent class
|   |   + example.py     # Example implementations
|   + api/
|       + __init__.py
|       + endpoints.py    # API routes
+ tests/
|   + test_registry.py
+ setup.py
+ requirements.txt
+ README.md
\end{verbatim}

\subsection{Testing Setup}
\subsubsection{Test Configuration}
Create pytest.ini for test configuration:
\begin{verbatim}
[pytest]
asyncio_mode = auto
testpaths = tests
python_files = test_*.py
python_classes = Test*
python_functions = test_*
\end{verbatim}

\subsubsection{Sample Test}
Example test implementation:
\begin{verbatim}
# tests/test_registry.py
import pytest
from src.core.registry import AgentRegistry
from src.agents.example import HelloAgent
from src.core.llm import MockLLM

@pytest.mark.asyncio
async def test_registry():
    registry = AgentRegistry()
    agent1 = HelloAgent("agent1", ["hello"], MockLLM())
    agent2 = HelloAgent("agent2", ["hello"], MockLLM())
    
    await registry.register(agent1)
    await registry.register(agent2)
    
    assert await registry.get_agent("agent1") == agent1
    with pytest.raises(ValueError):
        await registry.get_agent("nonexistent")
\end{verbatim}

\subsection{Dependency Management}
\paragraph{Setup.py Configuration}
\begin{verbatim}
from setuptools import setup, find_packages

setup(
    name="maci",
    version="0.1",
    packages=find_packages(),
    install_requires=[
        "fastapi",
        "uvicorn",
        "pydantic",
        "python-jose[cryptography]",
        "passlib[bcrypt]",
        "pytest",
        "pytest-asyncio"
    ],
)
\end{verbatim}

\subsection{Future Extensions}
\subsubsection{Planned Components}
\begin{itemize}
\item Authentication and Authorization
\item Advanced LLM Integration
\item Message Queue System
\item Persistent Storage
\item Web Interface
\item Monitoring and Logging
\end{itemize}

\subsubsection{Considerations}
\begin{itemize}
\item Agent Authentication
\item Message Encryption
\item Rate Limiting
\item Input Validation
\item Error Handling
\end{itemize}

\subsection{Development Workflow}
\subsubsection{Local Development}
\begin{enumerate}
\item Clone repository
\item Create virtual environment
\item Install dependencies
\item Run tests
\item Start development server
\end{enumerate}

\subsubsection{Adding New Agents}
Steps for implementing new agent types:
\begin{enumerate}
\item Create new agent class inheriting from BaseAgent
\item Implement process\_message method
\item Add specialized capabilities
\item Register with AgentRegistry
\item Add corresponding tests
\end{enumerate}

\subsection{API Documentation}
\paragraph{Endpoints}
\begin{itemize}
\item POST /agent/register
    \begin{itemize}
    \item Registers new agent
    \item Requires agent\_id and capabilities
    \item Returns success/failure status
    \end{itemize}
\item POST /agent/message
    \begin{itemize}
    \item Sends message to agent
    \item Requires source\_id, target\_id, message\_type, content
    \item Returns agent response
    \end{itemize}
\end{itemize}

\subsection{Error Handling}
\paragraph{Common Errors}
\begin{itemize}
\item Agent not found (404)
\item Invalid message format (422)
\item Duplicate agent registration (400)
\item Unsupported message type (400)
\end{itemize}

\subsection{Best Practices}
\begin{itemize}
\item Use type hints consistently
\item Document all public methods
\item Write tests for new functionality
\item Follow FastAPI conventions
\item Implement proper error handling
\item Use async/await correctly
\end{itemize}
