# Supplementary material for: MACI: Multi-Agent Collaborative Intelligence for Adaptive Reasoning and Temporal Planning
Source: arXiv:2501.16689 source file (2025-01-29)
Supplement: Supplementary file 4 [file AppendixOtherTexts.tex]

%\subsection{Tier 3: System Infrastructure (MAS)}

%We use MAS be our system infrastructure. Besides agent registration, search,
%and verification, we define communication protocols for agents to 
%communicate with each other.

%\subsubsection{Communication Protocol}
%Agents interact through a shared message space using a standardized format:
%\begin{equation}
%M = \{(a_i, a_j, t, c, p)\}
%\end{equation}
%where $a_i$ represents the source agent, $a_j$ the target agent, $t$ denotes message type (constraint, validation, update), $c$ represents content, and $p$ indicates priority level. The system implements asynchronous message passing with priority queues to optimize communication flow.

Planning systems require clear definitions of states and transitions to operate effectively. Table~\ref{tab:state_space} presents five fundamental state dimensions that form the basis of any planning task. Let us examine how these dimensions manifest themselves in real planning scenarios and how specialized agents operate on them.

The dimension \emph{Who} tracks the actors and their roles in the planning space. An actor's state includes not just their identity but their current roles and capabilities. In travel planning, a person might transition from driver to passenger, each role carrying specific constraints. A driver must maintain valid credentials and rest periods, while a passenger faces different constraints. The Role Manager Agent tracks these state transitions and ensures that role constraints remain satisfied.

The location states in the dimension \emph{Where} represent both physical and logical positions. Physical locations map to coordinates or addresses, while logical locations might represent stages in a process. The Navigation Agent in travel planning converts abstract location states (``airport,'' ``hotel'') into concrete coordinates and validates transitions between them. For financial planning, the Asset Location Agent tracks instrument positions across accounts and markets.

Temporal states capture both specific time points and the durations between them. The dimension \emph{When} allows planning systems to reason about deadlines and completion probabilities. Schedule Agents specialize these temporal states for domain requirements, coordinating flight connections in travel planning, or managing market hours and settlement periods in financial systems.

The resource states in the \emph{What} dimension track the available methods and their constraints. A travel Resource Agent manages transportation options and accommodations, while an Investment Agent handles financial instruments and capital allocation. Each maintains awareness of capacity limits and tracks associated costs.

The dimension \emph{Why} preserves the rationale of decisions and dependencies, allowing systems to explain their choices and adapt to changes. Strategy agents specialize in this dimension to maintain consistency with domain-specific goals and risk profiles.

\subsubsection{Agent Coordination and State Management}

Planning systems require continuous coordination between agents operating on different state dimensions. Consider how states evolve in a travel planning scenario: when a Schedule Agent identifies a flight connection constraint, it triggers state updates that ripple across multiple dimensions. The Location Agent must verify the feasibility of moving between terminals, while the Resource Agent checks transportation availability. The Role Manager Agent ensures travelers can meet their obligations at both origin and destination points.

This coordination happens through a state transition protocol. When any agent proposes a state change, it initiates a validation sequence:
\vspace{-.1in}
\begin{equation}
T: S_t \rightarrow S_{t+1} \text{ subject to } C_{\text{global}} \land C_{\text{local}}
\vspace{-.1in}
\end{equation}

where $S_t$ represents the current state vector across all dimensions, $S_{t+1}$ is the proposed new state, $C_{\text{global}}$ represents system-wide constraints, and $C_{\text{local}}$ captures domain-specific requirements.

\subsubsection{Agent Coordination for Validation}

The validation agent orchestrates the process by decomposing global constraints into dimension-specific checks. When a state change occurs, such as booking a flight, the validation agent initiates checks across multiple dimensions. These checks verify temporal constraints through the temporal agent, which examines connection times and arrival deadlines. The spatial agent validates terminal distances and transportation access, while the resource agent confirms seat availability and budget limits. The role agent ensures traveler availability meets duty limits.

State transitions in financial planning follow similar validation patterns with domain specialization. When investment agent proposes a trade, timing agent verifies market hours and settlement rules. The portfolio agent checks the position limits and balance requirements, while the strategy agent validates the risk tolerance and the alignment of the goals.

Common-sense agent serves as a critical component by identifying implicit constraints that domain agents might overlook. In travel scenarios, it identifies necessary rest periods between connections that other agents might miss. For financial planning, it recognizes unusual market conditions requiring additional validation steps. This layer of practical knowledge complements the formal constraints managed by specialized agents.
