# Supplementary material for: MACI: Multi-Agent Collaborative Intelligence for Adaptive Reasoning and Temporal Planning
Source: arXiv:2501.16689 source file (2025-01-29)
Supplement: Supplementary file 5 [file AppendixTSPApproximate.tex]

\section*{Heuristic $\mathbf{W^*}$ Framework for TSP}

\subsection*{Revised $\mathbf{W^*}$ Components}

\paragraph{Nodes}
\[
N = \{n_{\text{init}}, n_{\text{optimize}}, n_{\text{valid}}\}
\]
\begin{itemize}[leftmargin=1.5em]
    \item $n_{\text{init}}$: Initial solution generation (random/pheromone-based)
    \item $n_{\text{optimize}}$: Solution improvement via metaheuristics
    \item $n_{\text{valid}}$: Feasibility checking
\end{itemize}

\paragraph{Edges}
\[
E = \{e_{\text{fitness}}, e_{\text{penalty}}, e_{\text{converge}}\}
\]
\begin{itemize}[leftmargin=1.5em]
    \item $e_{\text{fitness}}$: Guides search using objective values
    \item $e_{\text{penalty}}$: Applies soft constraints
    \item $e_{\text{converge}}$: Monitors termination criteria
\end{itemize}

\paragraph{Agents}
\begin{itemize}[leftmargin=1.5em]
    \item \textbf{Node Agents}:
    \begin{itemize}
        \item Population Initializer (GA/ACO)
        \item Neighborhood Explorer (SA)
        \item Pheromone Updater (ACO)
    \end{itemize}
    \item \textbf{Edge Agents}:
    \begin{itemize}
        \item Fitness Calculator
        \item Constraint Penalizer ($\lambda$ tuning)
        \iteration Terminator
    \end{itemize}
\end{itemize}

\paragraph{Validation Function}
\[
V(W, M) = \begin{cases}
\text{fitness}(M) & \text{if feasible} \\
\text{fitness}(M) + \lambda \sum \text{violations}(M) & \text{otherwise}
\end{cases}
\]

\subsection*{Genetic Algorithm Implementation}

\begin{enumerate}[leftmargin=2em]
    \item \textbf{Initialization ($n_{\text{init}}$)}: Generate population of 100 random tours
    \item \textbf{Fitness ($e_{\text{fitness}}$)}: Calculate tour lengths
    \item \textbf{Optimization ($n_{\text{optimize}}$)}:
    \begin{itemize}
        \item Crossover: Edge recombination operator
        \item Mutation: 2-opt local search
        \item Selection: Tournament selection
    \end{itemize}
    \item \textbf{Validation ($n_{\text{valid}}$)}: Remove tours missing locations
    \item \textbf{Convergence ($e_{\text{converge}}$)}: Stop after 200 generations
\end{enumerate}

\subsection*{Simulated Annealing Implementation}

\begin{enumerate}[leftmargin=2em]
    \item \textbf{Initialization ($n_{\text{init}}$)}: Random tour $A\rightarrow C\rightarrow E\rightarrow D\rightarrow B\rightarrow A$
    \item \textbf{Optimization ($n_{\text{optimize}}$)}: 
    \begin{itemize}
        \item Neighborhood move: Reverse subtour
        \item Cooling schedule: $T_{k+1} = 0.95T_k$
    \end{itemize}
    \item \textbf{Fitness ($e_{\text{fitness}}$)}: Accept worse solutions with probability:
    \[
    P = \exp\left(-\frac{\Delta E}{T}\right)
    \]
    \item \textbf{Convergence ($e_{\text{converge}}$)}: Terminate at $T < 0.1$
\end{enumerate}

\subsection*{Ant Colony Optimization Implementation}

\begin{enumerate}[leftmargin=2em]
    \item \textbf{Initialization ($n_{\text{init}}$)}: 
    \[
    \tau_{ij}(0) = 0.1 \quad \forall (i,j)
    \]
    \item \textbf{Optimization ($n_{\text{optimize}}$)}:
    \begin{itemize}
        \item Path selection probability:
        \[
        P_{ij} = \frac{[\tau_{ij}]^\alpha [\eta_{ij}]^\beta}{\sum_{k} [\tau_{ik}]^\alpha [\eta_{ik}]^\beta}
        \]
        \item Pheromone update ($\rho=0.1$):
        \[
        \tau_{ij} \leftarrow (1-\rho)\tau_{ij} + \sum_{k=1}^m \Delta\tau_{ij}^k
        \]
    \end{itemize}
    \item \textbf{Validation ($n_{\text{valid}}$)}: Repair invalid paths
    \item \textbf{Convergence ($e_{\text{converge}}$)}: Stop after 50 cycles
\end{enumerate}

\subsection*{Performance Comparison}

\begin{center}
\begin{tabular}{lcc}
\toprule
Method & Complexity & Solution Quality \\
\midrule
Brute Force & $\mathcal{O}(n!)$ & Optimal \\
Genetic Algorithm & $\mathcal{O}(g \cdot p)$ & $\approx$95\% optimal \\
Simulated Annealing & $\mathcal{O}(k)$ & $\approx$90\% optimal \\
Ant Colony & $\mathcal{O}(c \cdot m \cdot n^2)$ & $\approx$97\% optimal \\
\bottomrule
\end{tabular}
\end{center}
\smallskip
\footnotesize Parameters: $g$=generations, $p$=population, $k$=iterations, $c$=cycles, $m$=ants

\vspace{1em}
\boxed{\text{Revised } \mathbf{W^*} \text{ enables polynomial-time heuristic TSP solving}}
