# Supplementary material for: MACI: Multi-Agent Collaborative Intelligence for Adaptive Reasoning and Temporal Planning
Source: arXiv:2501.16689 source file (2025-01-29)
Supplement: Supplementary file 6 [file AppendixERunTime.tex]

\section{MACI Execution Framework}
\label{app:MACIRunTime}

\subsection{Initialization}
\begin{itemize}[leftmargin=1.2em, topsep=-.2em, parsep=-.2em]
\item Load workflow $\mathbf{W}^*$ from meta-planner
\item Initialize required agents
\item Establish communication channels
\item Set up monitoring systems
\end{itemize}

\subsection{Execution Management}
The runtime manages workflow execution through:
\begin{equation}
\text{STN} = (V, E, w),
\end{equation}
where $V$ represents execution points, $E$ denotes dependencies, and $w$ indicates timing constraints.

\subsection{Monitoring and Validation}
Runtime validation operates at three levels:
\begin{itemize}[leftmargin=1.2em, topsep=-.2em, parsep=-.2em]
    \item Agent-level: Internal consistency checks
    \item System-level: Cross-agent validation
    \item Global-level: Overall workflow monitoring
\end{itemize}

\subsection{Dynamic Adjustment}
The runtime supports: real-time constraint updates,
resource reallocation, and workflow modification when needed

This execution framework ensures the theoretically constructed workflow can operate effectively in practice.
